# Supplementary material for: Niobium's intrinsic coherence length and penetration depth revisited using low-energy muon spin spectroscopy and secondary-ion mass spectrometry
Source: arXiv:2511.02913 source file (2026-01-14)
Supplement: Supplementary file 2 [file results-direct-local.tex]

\begin{tabular*}{\textwidth}{l @{\extracolsep{\fill}} S S S S S S}
\botrule
{Sample} & {$\ell$ (nm)} & {$T$ (\si{\kelvin})} & {$\tilde{B}_{0}$ (\si{\milli\tesla})} & {$d$ (\si{\nano\meter})} & {$\lambda(T)$ (\si{\nano\meter})} & {$\lambda_{0}$ (\si{\nano\meter})} \\
\hline
Nb-SR12 & 30.2 \pm 2.9 & 3.02 & 262.8 \pm 0.4 & 13.71 \pm 0.14 & 57.41 \pm 0.12 & 57.08 \pm 0.12 \\
Nb-SR13 & 380 \pm 40 & 3.00 & 259.4 \pm 0.4 & 16.28 \pm 0.12 & 32.73 \pm 0.07 & 32.55 \pm 0.07 \\
Nb-SR14 & 33.3 \pm 2.6 & 3.00 & 260.70 \pm 0.26 & 14.82 \pm 0.14 & 51.47 \pm 0.11 & 51.18 \pm 0.11 \\
Nb-SR15 & 13.6 \pm 1.2 & 3.02 & 263.0 \pm 0.4 & 13.66 \pm 0.17 & 68.40 \pm 0.21 & 68.01 \pm 0.21 \\
Nb-SR16 & 18.8 \pm 1.5 & 3.00 & 260.78 \pm 0.26 & 14.51 \pm 0.13 & 59.68 \pm 0.20 & 59.35 \pm 0.20 \\
Nb-SR18 & 69 \pm 5 & 3.04 & 261.3 \pm 0.4 & 14.66 \pm 0.14 & 43.02 \pm 0.11 & 42.77 \pm 0.12 \\

\botrule
\end{tabular*}
