# Supplementary material for: Niobium's intrinsic coherence length and penetration depth revisited using low-energy muon spin spectroscopy and secondary-ion mass spectrometry
Source: arXiv:2511.02913 source file (2026-01-14)
Supplement: Supplementary file 3 [file results-direct-nonlocal.tex]

\begin{tabular*}{\textwidth}{l @{\extracolsep{\fill}} S S S S S S}
\botrule
{Sample} & {$\ell$ (nm)} & {$T$ (\si{\kelvin})} & {$\tilde{B}_{0}$ (\si{\milli\tesla})} & {$d$ (\si{\nano\meter})} & {$\lambda_{L}$ (\si{\nano\meter})} & {$\xi_{0}$ (\si{\nano\meter})} \\
\hline
Nb-SR12 & 30.2 \pm 2.9 & 3.02 & 262.73 \pm 0.21 & 13.0719 \pm 0.0024 & 31.92 \pm 0.05 & 39.7243 \pm 0.0028 \\
Nb-SR13 & 380 \pm 40 & 2.99 & 261.05 \pm 0.04 & 13.00 \pm 0.17 & 28.508 \pm 0.008 & 39.98 \pm 0.26 \\
Nb-SR14 & 33.3 \pm 2.6 & 3.00 & 261.64 \pm 0.18 & 13.68650 \pm 0.00024 & 29.86 \pm 0.04 & 38.7738 \pm 0.0008 \\
Nb-SR15 & 13.6 \pm 1.2 & 3.02 & 260.15 \pm 0.21 & 15.00 \pm 0.06 & 28.34 \pm 0.05 & 38.9254 \pm 0.0018 \\
Nb-SR16 & 18.8 \pm 1.5 & 3.00 & 260.75 \pm 0.18 & 14.5008 \pm 0.0022 & 26.23 \pm 0.04 & 32.275 \pm 0.004 \\
Nb-SR18 & 69 \pm 5 & 3.04 & 264.17 \pm 0.08 & 12.49 \pm 0.23 & 30.247 \pm 0.019 & 39.5 \pm 0.6 \\
\hline
 & & & & & 29.2 \pm 2.0 & 38.2 \pm 2.9 \\
\botrule
\end{tabular*}
