# Supplementary material for: Niobium's intrinsic coherence length and penetration depth revisited using low-energy muon spin spectroscopy and secondary-ion mass spectrometry
Source: arXiv:2511.02913 source file (2026-01-14)
Supplement: Supplementary file 4 [file results-staged-local.tex]

\begin{tabular*}{\textwidth}{l @{\extracolsep{\fill}} S S S S S S S}
\botrule
{Sample} & {$\ell$ (nm)} & {$T$ (\si{\kelvin})} & {$B_{\mathrm{applied}}$ (\si{\milli\tesla})} & {$\tilde{N}$} & {$d$ (\si{\nano\meter})} & {$\lambda(T)$ (\si{\nano\meter})} & {$\lambda_{0}$ (\si{\nano\meter})} \\
\hline
Nb-SR12 & 30.2 \pm 2.9 & 3.02 &  \dots  &  \dots  & 13.2 \pm 0.5 & 56.9 \pm 1.2 & 56.6 \pm 1.2 \\
Nb-SR13 & 380 \pm 40 & 2.99 &  \dots  &  \dots  & 12.6 \pm 0.4 & 35.4 \pm 0.7 & 35.2 \pm 0.7 \\
Nb-SR14 & 33.3 \pm 2.6 & 3.00 & 25.1586 \pm 0.0016 & 0.051 \pm 0.004 & 12.5 \pm 0.5 & 54.7 \pm 1.4 & 54.4 \pm 1.4 \\
Nb-SR15 & 13.6 \pm 1.2 & 3.02 &  \dots  &  \dots  & 12.6 \pm 0.6 & 68.9 \pm 1.6 & 68.5 \pm 1.6 \\
Nb-SR16 & 18.8 \pm 1.5 & 3.00 &  \dots  &  \dots  & 13.0 \pm 0.5 & 63.6 \pm 1.3 & 63.3 \pm 1.3 \\
Nb-SR18 & 69 \pm 5 & 3.04 &  \dots  &  \dots  & 14.3 \pm 0.4 & 43.5 \pm 1.1 & 43.3 \pm 1.1 \\

\botrule
\end{tabular*}
