# Supplementary material for: Niobium's intrinsic coherence length and penetration depth revisited using low-energy muon spin spectroscopy and secondary-ion mass spectrometry
Source: arXiv:2511.02913 source file (2026-01-14)
Supplement: Supplementary file 5 [file results-staged-nonlocal.tex]

\begin{tabular*}{\textwidth}{l @{\extracolsep{\fill}} S S S S S S S}
\botrule
{Sample} & {$\ell$ (nm)} & {$T$ (\si{\kelvin})} & {$B_{\mathrm{applied}}$ (\si{\milli\tesla})} & {$\tilde{N}$} & {$d$ (\si{\nano\meter})} & {$\lambda_{L}$ (\si{\nano\meter})} & {$\xi_{0}$ (\si{\nano\meter})} \\
\hline
Nb-SR12 & 30.2 \pm 2.9 & 3.02 &  \dots  &  \dots  & 12.4 \pm 0.6 &  \dots  &  \dots  \\
Nb-SR13 & 380 \pm 40 & 2.99 &  \dots  &  \dots  & 10.7 \pm 0.4 &  \dots  &  \dots  \\
Nb-SR14 & 33.3 \pm 2.6 & 3.00 & 25.1586 \pm 0.0016 & 0.059 \pm 0.005 & 11.6 \pm 0.6 & 29.0 \pm 1.2 & 45 \pm 5 \\
Nb-SR15 & 13.6 \pm 1.2 & 3.02 &  \dots  &  \dots  & 11.1 \pm 0.7 &  \dots  &  \dots  \\
Nb-SR16 & 18.8 \pm 1.5 & 3.00 &  \dots  &  \dots  & 11.9 \pm 0.6 &  \dots  &  \dots  \\
Nb-SR18 & 69 \pm 5 & 3.04 &  \dots  &  \dots  & 12.9 \pm 0.5 &  \dots  &  \dots  \\

\botrule
\end{tabular*}
