# Supplementary material for: Niobium's intrinsic coherence length and penetration depth revisited using low-energy muon spin spectroscopy and secondary-ion mass spectrometry
Source: arXiv:2511.02913 source file (2026-01-14)
Supplement: Supplementary file 6 [file sims-results-summary.tex]

\begin{ruledtabular}
\begin{tabular}{l S l l S S S S}
{SIMS Sample} & {Depth (\unit{\nano\meter})} & {LE-$\mu$SR Sample} & {Trial} & {[\ch{C}] (\unit{ppma})} & {[\ch{N}] (\unit{ppma})} & {[\ch{O}] (\unit{ppma})} & {$\ell$ (\unit{\nano\meter})}  \\
\hline
Nb-SR1 & 300 & Nb-SR14 & \emph{Combined} & 115 \pm 11 & 45.4 \pm 2.9 & 2310 \pm 120 & 33.3 \pm 2.6 \\[1.5ex]
Nb-SR2 & 300 & Nb-SR15 & \emph{Combined} & 154.1 \pm 3.1 & 41.3 \pm 3.3 & 5840 \pm 350 & 13.6 \pm 1.2 \\[1.5ex]
Nb-SR3 & 300 & Nb-SR16 & \emph{Combined} & 127 \pm 6 & 43.0 \pm 2.8 & 4400 \pm 90 & 18.0 \pm 1.2 \\[1.5ex]
 & 1000 & Nb-SR12 & \emph{Combined} & 128 \pm 7 & 53 \pm 10 & 2720 \pm 90 & 28.3 \pm 2.0 \\[1.5ex]
 & 4800 & Nb-SR13 & \emph{Combined} & 118 \pm 4 & 53 \pm 7 & 51.8 \pm 1.1 & 365 \pm 24 \\[1.5ex]
Nb-SR4 & 300 & Nb-SR18 & \emph{Combined} & 101 \pm 6 & 46.2 \pm 3.2 & 1041 \pm 34 & 69 \pm 5 \\[1.5ex]
Nb-SR8 & 300 & Nb-SR16 & \emph{Combined} & 126 \pm 23 & 48.8 \pm 2.4 & 4040 \pm 120 & 19.5 \pm 1.4 \\[1.5ex]
 & 1000 & Nb-SR12 & \emph{Combined} & 119 \pm 22 & 55 \pm 8 & 2370 \pm 60 & 32.3 \pm 2.2 \\[1.5ex]
 & 4800 & Nb-SR13 & \emph{Combined} & 108 \pm 22 & 47.6 \pm 2.6 & 48 \pm 7 & 400 \pm 50 \\[1.5ex]
\hline \\[0.5ex]
Nb-SR3 + Nb-SR8 & 300 & Nb-SR16 & \emph{Combined} & 127 \pm 18 & 46 \pm 4 & 4200 \pm 210 & 18.8 \pm 1.5 \\[1.5ex]
 & 1000 & Nb-SR12 & \emph{Combined} & 123 \pm 17 & 54 \pm 9 & 2540 \pm 190 & 30.2 \pm 2.9 \\[1.5ex]
 & 4800 & Nb-SR13 & \emph{Combined} & 113 \pm 18 & 51 \pm 7 & 50 \pm 5 & 380 \pm 40 \\
\end{tabular}
\end{ruledtabular}
