# Supplementary material for: Niobium's intrinsic coherence length and penetration depth revisited using low-energy muon spin spectroscopy and secondary-ion mass spectrometry
Source: arXiv:2511.02913 source file (2026-01-14)
Supplement: Supplementary file 7 [file stopping-pars.tex]

\begin{tabular*}{\textwidth}{S @{\extracolsep{\fill}} S S S S S S S}
\botrule
{$E$ (\unit{\kilo\electronvolt})} & {$\alpha_{1}$} & {$\beta_{1}$} & {$z_{\mathrm{max},1}$ (\unit{\nano\meter})} & {$f_{1}$} & {$\alpha_{2}$} & {$\beta_{2}$} & {$z_{\mathrm{max},2}$ (\unit{\nano\meter})} \\
\hline
0.5 & 3.47 \pm 0.06 & 13.8 \pm 0.6 & 32.5 \pm 0.8 & 0.828 \pm 0.004 & 1.736 \pm 0.020 & 3.01 \pm 0.10 & 4.41 \pm 0.08 \\
1.0 & 3.381 \pm 0.023 & 8.56 \pm 0.13 & 29.31 \pm 0.20 & 0.9195 \pm 0.0012 & 1.797 \pm 0.022 & 2.49 \pm 0.07 & 4.21 \pm 0.04 \\
1.5 & 4.67 \pm 0.05 & 9.20 \pm 0.25 & 33.4 \pm 0.4 & 0.598 \pm 0.010 & 1.683 \pm 0.009 & 3.02 \pm 0.06 & 22.29 \pm 0.08 \\
2.0 & 4.646 \pm 0.034 & 7.08 \pm 0.08 & 33.90 \pm 0.15 & 0.582 \pm 0.005 & 1.695 \pm 0.010 & 2.234 \pm 0.025 & 23.054 \pm 0.027 \\
2.5 & 5.00 \pm 0.04 & 6.52 \pm 0.07 & 36.04 \pm 0.12 & 0.555 \pm 0.005 & 1.764 \pm 0.010 & 2.144 \pm 0.020 & 25.992 \pm 0.024 \\
3.0 & 5.10 \pm 0.04 & 5.82 \pm 0.05 & 37.98 \pm 0.08 & 0.530 \pm 0.004 & 1.769 \pm 0.010 & 1.891 \pm 0.017 & 27.929 \pm 0.017 \\
3.5 & 5.86 \pm 0.05 & 6.12 \pm 0.05 & 40.96 \pm 0.09 & 0.501 \pm 0.004 & 1.863 \pm 0.009 & 1.985 \pm 0.016 & 30.964 \pm 0.019 \\
4.0 & 6.58 \pm 0.05 & 6.33 \pm 0.05 & 43.70 \pm 0.07 & 0.482 \pm 0.004 & 1.952 \pm 0.008 & 2.081 \pm 0.015 & 33.975 \pm 0.023 \\
4.5 & 6.45 \pm 0.05 & 5.66 \pm 0.06 & 45.21 \pm 0.10 & 0.493 \pm 0.004 & 1.944 \pm 0.008 & 1.962 \pm 0.015 & 35.938 \pm 0.020 \\
5.0 & 6.62 \pm 0.05 & 5.40 \pm 0.05 & 47.34 \pm 0.09 & 0.494 \pm 0.004 & 1.955 \pm 0.008 & 1.901 \pm 0.015 & 37.933 \pm 0.019 \\
5.5 & 7.18 \pm 0.05 & 5.75 \pm 0.06 & 50.21 \pm 0.10 & 0.488 \pm 0.004 & 1.979 \pm 0.008 & 1.918 \pm 0.013 & 40.925 \pm 0.020 \\
6.0 & 7.21 \pm 0.05 & 5.46 \pm 0.05 & 52.23 \pm 0.09 & 0.489 \pm 0.004 & 1.999 \pm 0.008 & 1.857 \pm 0.013 & 42.901 \pm 0.018 \\
6.5 & 7.29 \pm 0.05 & 5.29 \pm 0.04 & 54.28 \pm 0.08 & 0.4979 \pm 0.0035 & 1.980 \pm 0.008 & 1.786 \pm 0.012 & 44.870 \pm 0.017 \\
7.0 & 7.95 \pm 0.05 & 5.57 \pm 0.04 & 56.70 \pm 0.08 & 0.523 \pm 0.004 & 2.070 \pm 0.008 & 2.059 \pm 0.014 & 48.848 \pm 0.029 \\
7.5 & 7.60 \pm 0.05 & 5.24 \pm 0.04 & 59.02 \pm 0.07 & 0.4955 \pm 0.0032 & 1.989 \pm 0.008 & 1.665 \pm 0.011 & 48.839 \pm 0.014 \\
8.0 & 7.37 \pm 0.05 & 4.79 \pm 0.04 & 60.39 \pm 0.08 & 0.5230 \pm 0.0033 & 1.970 \pm 0.008 & 1.642 \pm 0.011 & 50.821 \pm 0.014 \\
8.5 & 5.77 \pm 0.04 & 2.813 \pm 0.017 & 55.30 \pm 0.04 & 0.589 \pm 0.004 & 1.934 \pm 0.009 & 1.954 \pm 0.009 & 58.908 \pm 0.024 \\
9.0 & 5.78 \pm 0.05 & 2.660 \pm 0.017 & 56.168 \pm 0.035 & 0.542 \pm 0.004 & 1.881 \pm 0.010 & 1.571 \pm 0.007 & 58.837 \pm 0.014 \\
9.5 & 6.03 \pm 0.04 & 2.782 \pm 0.017 & 59.16 \pm 0.04 & 0.568 \pm 0.004 & 1.920 \pm 0.009 & 1.709 \pm 0.008 & 61.903 \pm 0.019 \\
10.0 & 5.80 \pm 0.04 & 2.556 \pm 0.016 & 60.131 \pm 0.032 & 0.556 \pm 0.004 & 1.856 \pm 0.010 & 1.467 \pm 0.007 & 62.767 \pm 0.011 \\
10.5 & 6.09 \pm 0.04 & 2.696 \pm 0.016 & 63.16 \pm 0.04 & 0.580 \pm 0.004 & 1.902 \pm 0.009 & 1.599 \pm 0.007 & 65.836 \pm 0.016 \\
11.0 & 6.11 \pm 0.04 & 2.650 \pm 0.015 & 65.15 \pm 0.04 & 0.585 \pm 0.004 & 1.887 \pm 0.009 & 1.541 \pm 0.007 & 67.795 \pm 0.014 \\
11.5 & 6.08 \pm 0.04 & 2.590 \pm 0.015 & 67.172 \pm 0.034 & 0.592 \pm 0.004 & 1.878 \pm 0.010 & 1.500 \pm 0.007 & 69.782 \pm 0.013 \\
12.0 & 6.42 \pm 0.04 & 2.726 \pm 0.015 & 70.08 \pm 0.04 & 0.6062 \pm 0.0034 & 1.945 \pm 0.009 & 1.626 \pm 0.007 & 72.843 \pm 0.018 \\
12.5 & 6.41 \pm 0.04 & 2.670 \pm 0.014 & 72.11 \pm 0.04 & 0.6144 \pm 0.0033 & 1.926 \pm 0.010 & 1.572 \pm 0.007 & 74.814 \pm 0.016 \\
13.0 & 6.75 \pm 0.04 & 2.810 \pm 0.016 & 75.05 \pm 0.05 & 0.6271 \pm 0.0031 & 1.979 \pm 0.009 & 1.703 \pm 0.008 & 77.895 \pm 0.023 \\
13.5 & 6.68 \pm 0.04 & 2.743 \pm 0.015 & 77.02 \pm 0.05 & 0.6350 \pm 0.0031 & 1.950 \pm 0.009 & 1.626 \pm 0.008 & 79.845 \pm 0.020 \\
14.0 & 6.68 \pm 0.04 & 2.685 \pm 0.013 & 79.24 \pm 0.04 & 0.6498 \pm 0.0029 & 1.98 \pm 0.01 & 1.704 \pm 0.008 & 82.812 \pm 0.021 \\
14.5 & 6.85 \pm 0.04 & 2.778 \pm 0.014 & 82.20 \pm 0.04 & 0.6733 \pm 0.0027 & 1.999 \pm 0.010 & 1.813 \pm 0.009 & 85.848 \pm 0.027 \\
15.0 & 6.94 \pm 0.04 & 2.739 \pm 0.013 & 84.18 \pm 0.04 & 0.6670 \pm 0.0027 & 2.013 \pm 0.010 & 1.757 \pm 0.008 & 87.860 \pm 0.026 \\
15.5 & 7.04 \pm 0.04 & 2.808 \pm 0.014 & 87.11 \pm 0.05 & 0.6873 \pm 0.0027 & 2.023 \pm 0.010 & 1.839 \pm 0.009 & 90.814 \pm 0.029 \\
16.0 & 7.10 \pm 0.04 & 2.764 \pm 0.013 & 89.15 \pm 0.05 & 0.6847 \pm 0.0026 & 2.015 \pm 0.010 & 1.765 \pm 0.008 & 92.832 \pm 0.027 \\
16.5 & 7.28 \pm 0.04 & 2.824 \pm 0.017 & 91.89 \pm 0.07 & 0.6988 \pm 0.0025 & 2.048 \pm 0.010 & 1.861 \pm 0.011 & 95.820 \pm 0.033 \\
17.0 & 7.33 \pm 0.04 & 2.798 \pm 0.013 & 94.21 \pm 0.04 & 0.7070 \pm 0.0024 & 2.051 \pm 0.010 & 1.896 \pm 0.009 & 98.753 \pm 0.029 \\
17.5 & 7.29 \pm 0.04 & 2.731 \pm 0.012 & 96.27 \pm 0.04 & 0.7034 \pm 0.0024 & 2.061 \pm 0.010 & 1.821 \pm 0.008 & 100.760 \pm 0.027 \\
18.0 & 7.52 \pm 0.04 & 2.799 \pm 0.013 & 99.11 \pm 0.05 & 0.7125 \pm 0.0024 & 2.102 \pm 0.010 & 1.902 \pm 0.009 & 103.771 \pm 0.032 \\
18.5 & 7.61 \pm 0.04 & 2.844 \pm 0.015 & 101.94 \pm 0.07 & 0.7291 \pm 0.0023 & 2.093 \pm 0.010 & 1.968 \pm 0.011 & 106.77 \pm 0.04 \\
19.0 & 7.589 \pm 0.035 & 2.775 \pm 0.012 & 104.05 \pm 0.05 & 0.7266 \pm 0.0022 & 2.071 \pm 0.010 & 1.857 \pm 0.009 & 108.744 \pm 0.030 \\
19.5 & 7.69 \pm 0.04 & 2.804 \pm 0.016 & 106.83 \pm 0.08 & 0.7359 \pm 0.0022 & 2.082 \pm 0.010 & 1.913 \pm 0.011 & 111.720 \pm 0.033 \\
20.0 & 7.79 \pm 0.04 & 2.781 \pm 0.012 & 109.16 \pm 0.05 & 0.7311 \pm 0.0022 & 2.091 \pm 0.010 & 1.848 \pm 0.009 & 113.755 \pm 0.031 \\
20.5 & 7.672 \pm 0.035 & 2.684 \pm 0.011 & 111.29 \pm 0.04 & 0.7366 \pm 0.0022 & 2.098 \pm 0.010 & 1.841 \pm 0.008 & 116.680 \pm 0.025 \\
21.0 & 7.83 \pm 0.04 & 2.734 \pm 0.011 & 114.25 \pm 0.04 & 0.7457 \pm 0.0021 & 2.115 \pm 0.010 & 1.898 \pm 0.009 & 119.638 \pm 0.025 \\
21.5 & 7.763 \pm 0.035 & 2.640 \pm 0.011 & 116.24 \pm 0.04 & 0.7391 \pm 0.0021 & 2.094 \pm 0.010 & 1.780 \pm 0.008 & 121.686 \pm 0.024 \\
22.0 & 7.92 \pm 0.04 & 2.675 \pm 0.011 & 119.05 \pm 0.05 & 0.7365 \pm 0.0022 & 2.094 \pm 0.010 & 1.730 \pm 0.008 & 123.711 \pm 0.026 \\
22.5 & 7.89 \pm 0.04 & 2.595 \pm 0.010 & 121.11 \pm 0.04 & 0.7286 \pm 0.0022 & 2.071 \pm 0.010 & 1.619 \pm 0.007 & 125.713 \pm 0.022 \\
23.0 & 7.964 \pm 0.035 & 2.627 \pm 0.010 & 124.28 \pm 0.04 & 0.7478 \pm 0.0020 & 2.094 \pm 0.010 & 1.739 \pm 0.008 & 129.672 \pm 0.024 \\
23.5 & 8.14 \pm 0.04 & 2.659 \pm 0.010 & 127.15 \pm 0.04 & 0.7504 \pm 0.0020 & 2.114 \pm 0.010 & 1.765 \pm 0.008 & 132.646 \pm 0.023 \\
24.0 & 8.10 \pm 0.04 & 2.572 \pm 0.010 & 129.16 \pm 0.04 & 0.7343 \pm 0.0021 & 2.063 \pm 0.010 & 1.566 \pm 0.007 & 133.685 \pm 0.020 \\
24.5 & 8.147 \pm 0.035 & 2.589 \pm 0.010 & 132.23 \pm 0.04 & 0.7502 \pm 0.0020 & 2.10 \pm 0.01 & 1.674 \pm 0.007 & 137.672 \pm 0.022 \\
25.0 & 8.46 \pm 0.04 & 2.705 \pm 0.012 & 135.90 \pm 0.06 & 0.7613 \pm 0.0020 & 2.172 \pm 0.011 & 1.830 \pm 0.009 & 141.634 \pm 0.026 \\
25.5 & 8.23 \pm 0.04 & 2.515 \pm 0.010 & 137.15 \pm 0.04 & 0.7370 \pm 0.0021 & 2.071 \pm 0.010 & 1.498 \pm 0.007 & 141.712 \pm 0.020 \\
26.0 & 8.26 \pm 0.04 & 2.521 \pm 0.009 & 140.24 \pm 0.04 & 0.7508 \pm 0.0020 & 2.089 \pm 0.011 & 1.581 \pm 0.007 & 145.648 \pm 0.019 \\
26.5 & 8.53 \pm 0.04 & 2.625 \pm 0.010 & 144.01 \pm 0.05 & 0.7617 \pm 0.0019 & 2.143 \pm 0.011 & 1.712 \pm 0.008 & 149.662 \pm 0.024 \\
27.0 & 8.63 \pm 0.04 & 2.636 \pm 0.010 & 147.00 \pm 0.05 & 0.7657 \pm 0.0019 & 2.155 \pm 0.011 & 1.714 \pm 0.008 & 152.671 \pm 0.026 \\
27.5 & 8.47 \pm 0.04 & 2.521 \pm 0.009 & 149.18 \pm 0.04 & 0.757 \pm 0.002 & 2.119 \pm 0.011 & 1.594 \pm 0.007 & 154.675 \pm 0.022 \\
28.0 & 8.62 \pm 0.04 & 2.536 \pm 0.009 & 152.16 \pm 0.04 & 0.7567 \pm 0.0019 & 2.126 \pm 0.011 & 1.579 \pm 0.007 & 157.656 \pm 0.020 \\
28.5 & 8.60 \pm 0.04 & 2.516 \pm 0.009 & 155.19 \pm 0.04 & 0.7621 \pm 0.0019 & 2.126 \pm 0.011 & 1.576 \pm 0.007 & 160.687 \pm 0.023 \\
29.0 & 8.75 \pm 0.04 & 2.522 \pm 0.009 & 158.03 \pm 0.04 & 0.7516 \pm 0.0020 & 2.123 \pm 0.011 & 1.497 \pm 0.007 & 162.684 \pm 0.020 \\
29.5 & 8.77 \pm 0.04 & 2.507 \pm 0.009 & 161.00 \pm 0.04 & 0.7551 \pm 0.0020 & 2.117 \pm 0.011 & 1.486 \pm 0.007 & 165.693 \pm 0.021 \\
30.0 & 8.90 \pm 0.04 & 2.507 \pm 0.009 & 163.94 \pm 0.05 & 0.751 \pm 0.002 & 2.124 \pm 0.011 & 1.457 \pm 0.007 & 168.692 \pm 0.020 \\
\botrule
\end{tabular*}
